# Supplementary material for: The structure of gene-gene networks beyond pairwise interactions
Source: arXiv:2111.08436 source file (2021-10-14)
Supplement: Supplementary file 1 [file suplementary.pdf]

***Essential genes with the most participation in balance of global network:***

| | | | | |
|---|---|---|---|---|
| YPR035W | YFR031C | YBR143C | YMR043W | YER168C |
| YBR121C | YIL147C | YDL030W | YOL146W | YLR060W |
| YPL083C | YJL054W | YDR182W | YDR303C | YBR153W |
| YPL231W | YPL231W | YDR141C | YER172C | YAL041W |

***Nonessential genes with the most participation in balance of global network:***

| | | | | |
|---|---|---|---|---|
| YMR175W | YCL074W | YDR528W | YHR049C-A | YOR006C |
| YLR294C | YLR431C | YML052W | YLR438W | YHR133C |
| YJR161C | YBR226C | YER085C | YPR003C | YBL054W |
| YLL016W | YML100W | YEL004W | YMR244C-A | YDR340W |
| YLR456W | YMR166C | YOR054C | YIR044C | YKL171W |
| YBR259W | YER090W | YBR020W | YBR199W | YDR401W |
| YJR058C | YHR124W | YDR497C | YOR263C | YOR051C |
| YKL034W | YGL230C | YPL191C | YIL058W | YLR303W |
| YGL060W | YLR351C | YKL091C | YGR059W | YBR206W |
| YGR203W | YLR090W | YLR247C | YOR107W | YKL044W |
| YDR371W | YHL024W | YML016C | YML057C-A | YGL260W |
| YPL023C | YPR199C | YKR090W | YJR091C | YML116W |
| YDR269C | YOR031W | YDR220C | YGL221C | YPR188C |
| YOR173W | YBR024W | YER134C | YER071C | YHR192W |
| YIL028W | YFL004W | YLR450W | YOR307C | YOR222W |
| YOR316C | YHR174W | YOL047C | YKL094W | YMR020W |
| YBR241C | YER182W | YJL199C | YDR248C | YLR084C |
| YHR093W | YDR035W | YBR224W | YJR092W | YIL067C |
| YJR082C | YJL055W | YML116W-A | YLR224W | YGL039W |
| YJL007C | YJL016W | YPL140C | YDR514C | YDR333C |
| YMR030W | YGR043C | YGR051C | YMR243C | YKL065C |
| YIL001W | YKL097C | YOR376W | YGL159W | YER188W |
| YOR015W | YKR045C | YHR021C | YMR037C | YOL025W |
| YPL249C | YPL224C | YOR248W | YLR142W | YPR140W |
| YLR422W | YBR172C | YER108C | YMR188C | YGL139W |
| YKR011C | YDR518W | YGL249W | YBR092C | YLR054C |
| YNL116W | YML038C | YOL086C | YHR199C | YIL009C-A |
| YHR113W | YAR042W | YNR040W | YLR257W | YPL021W |
| YLR233C | YIL168W | YHR014W | YDR319C | YGL089C |
| YKL096W-A | YMR221C | YBR249C | YDL054C | YDL154W |
| YGR100W | YBR299W | YHR150W | YJL217W | YOR033C |
| YPR154W | YNL046W | YJR070C | YHR210C | YMR219W |

| | | | | |
|---|---|---|---|---|
| YPR054W | YGL177W | YPR149W | YFR035C | YJR066W |
| YIL036W | YHL036W | YLR372W | YDL012C | YKL168C |
| YBR295W | YPR170C | YHR123W | YKR078W | YLR028C |
| YLR114C | YPL250C | YHR202W | YPL136W | YER180C |
| YMR007W | YBR213W | YHR134W | YCL006C | YOL075C |
| YIR001C | YAL045C | YLL046C | YMR019W | YLR237W |
| YDR275W | YMR103C | YKR072C | YIL131C | YOR366W |
| YOR252W | YOR338W | YDL001W | YER066C-A | YIL066C |
| YKL166C | YGL157W | YMR119W-A | YPR198W | YMR319C |
| YMR234W | YMR206W | YDR112W | YLR097C | YLR012C |
| YGR014W | YIL132C | YOL132W | YKL031W | YBR214W |
| YDR385W | YHR184W | YIL072W | YBR246W | YNL286W |
| YLR019W | YOR284W | YDL073W | YML047W-A | YDR330W |
| YDR058C | YIL055C | YHR022C | YER132C | YOL083W |
| YOR239W | YKR104W | YKL084W | YDL201W | YDR286C |
| YDL231C | YML011C | YFL034C-A | YKL057C | YPL208W |
| YFL006W | YNL083W | YHR008C | YMR141C | YPL221W |
| YHR043C | YOR108W | YLR149C | YOR016C | YKR103W |
| YDR384C | YPR172W | YOR223W | YOR356W | YIL045W |
| YDR272W | YBR219C | YPL105C | YDR379W | YOL098C |
| YGR012W | YER177W | YFR044C | YGL009C | YLR194C |
| YER046W | YLR279W | YDL078C | YJR059W | YMR167W |
| YDR305C | YIL092W | YOR393W | YAR043C | YER175C |
| YGL257C | YDR436W | YBR216C | YDR077W | YBR176W |
| YMR162C | YBR182C | YMR251W | YML075C | YPR059C |
| YHR178W | YMR289W | YIL014W | YBR158W | YOR028C |
| YDR402C | YJR047C | YLL062C | YKL102C | YPL189W |
| YOR105W | YNR056C | YOR175C | YBR222C | YMR027W |
| YPR038W | YPR098C | YDL094C | YOL029C | YAR037W |
| YHR161C | YER066W | YBR225W | YEL040W | YKL217W |
| YBR041W | YBR132C | YHL041W | YKL092C | YHL008C |
| YBR255C-A | YGR015C | YBR014C | YJL070C | YLR416C |
| YJR019C | YPR042C | YGL037C | YOR072W | YDR503C |
| YMR316C-A | YLR121C | YDL130W-A | YOL113W | YBL067C |
| YOR032C | YPL197C | YOR092W | YKL056C | YOR347C |
| YGR291C | YFL011W | YGR007W | YLR437C | YNL130C |
| YLR307W | YLR263W | YER067C-A | YDR006C | YDL144C |
| YER101C | YHR207C | YKR032W | YHR048W | YKR051W |
| YGR234W | YDR106W | YER091C | YOL045W | YPR193C |
| YCR076C | YDR524C | YLR434C | YKL030W | YKL202W |
| YMR192W | YMR172C-A | YLR346C | YMR196W | YDR144C |
| YGR021W | YDR294C | YIL171W | YLR365W | YNR021W |
| YBR183W | YIL012W | YLR020C | YDL123W | YIL027C |
| YPL019C | YJL215C | YOR128C | YIL101C | YGR236C |
| YCL005W | YJL057C | YLR036C | YJL142C | YOL117W |
| YGL232W | YDR099W | YMR105C | YCL038C | YLL047W |

| | | | | |
|---|---|---|---|---|
| YKR009C | YGL080W | YJL151C | YNL077W | YPL206C |
| YKR067W | YKL086W | YPL167C | YOL128C | YDL091C |
| YIL114C | YHL028W | YFR049W | YBL024W | YFL021W |
| YDL066W | YOR071C | YIR020W-A | YDR072C | YHR138C |
| YGL144C | YCR073C | YLR326W | YML056C | YMR321C |
| YIL024C | YLR449W | YMR261C | YKR089C | YOL046C |
| YOR137C | YLR001C | YPL116W | YML107C | YMR326C |
| YBR292C | YNL208W | YCR106W | YKL177W | YGR271W |
| YGL118C | YKL199C | YPR147C | YFL056C | YHL045W |
| YLR262C-A | YER183C | YHR095W | YLL025W | YIL086C |
| YAL066W | YDR411C | YLR400W | YNL095C | YOL017W |
| YDR312W | YKL067W | YGR137W | YEL038W | YPL096W |
| YER072W | YFL030W | YPR027C | YMR244W | YBR185C |
| YOR219C | YNL098C | YKR076W | YOR328W | YHL009C |
| YGR069W | YDR124W | YPR005C | YER150W | YLR152C |
| YOR377W | YMR313C | YOL160W | YDR516C | YDR511W |
| YMR245W | YIL052C | YHR136C | YGR290W | YHR163W |
| YLR246W | YIL032C | YOR118W | YHR182W | YBL081W |
| YDL174C | YDL191W | YMR173W-A | YOR171C | YGR123C |
| YER179W | YER062C | YPL135W | YFR020W | YLR124W |
| YPL092W | YHL022C | YBL039W-B | YIL137C | YDR122W |
| YFR053C | YOR301W | YBL001C | YCR083W | YOR292C |
| YLR253W | YPR061C | YKR077W | YDL236W | YER176W |
| YJL083W | YAR047C | YGR202C | YPR122W | YGR040W |
| YPR015C | YPR002W | YJL107C | YDR422C | YPL247C |
| YOL141W | YGR050C | YOR367W | YOR062C | YAL028W |
| YMR187C | YIR043C | YKL026C | YLR128W | YHR158C |
| YMR106C | YPL130W | YGR199W | YNL016W | YLR284C |
| YPR171W | YMR090W | YDR271C | YNL100W | YDR400W |
| YAL031C | YLL010C | YPL207W | YGL085W | YJL205C |
| YBR212W | YFL041W | YOR289W | YLL061W | YJL022W |
| YPR004C | YNL123W | YDL109C | YAL048C | YGL015C |
| YOL150C | YKR087C | YGL021W | YHR001W-A | YBR013C |
| YJR145C | YOR131C | YDR084C | YJL165C | YMR099C |
| YHR198C | YHR204W | YDR247W | YKR066C | YBR032W |
| YIL135C | YGR273C | YER188C-A | YBL088C | YGR178C |
| YLL052C | YPL186C | YHL040C | YFR054C | YIL099W |
| YDR475C | YOR059C | YFL007W | YGR242W | YMR259C |
| YHR130C | YFR056C | YIR036C | YAR030C | YGR110W |
| YDR242W | YFL015C | YLR356W | YER049W | YDR179C |
| YFL053W | YLR168C | YKL183W | YDR285W | YNL194C |
| YFR041C | YGR210C | YDL180W | YMR284W | YGL032C |
| YMR114C | YDR105C | YLL063C | YML059C | YDR403W |
| YPL072W | YBR043C | YAL051W | YLR443W | YKL071W |
| YIL122W | YGL189C | YBL032W | YGL062W | YHR032W |
| YMR209C | YHR144C | YGR177C | YER170W | YDL216C |

| | | | | |
|---|---|---|---|---|
| YLR280C | YGL053W | YOL131W | YER128W | YNR013C |
| YNL156C | YDR018C | YGR042W | YLR334C | YPL067C |
| YOR053W | YMR315W | YGR176W | YBR093C | YLR225C |
| YIL130W | YOL163W | YIR017C | YGL198W | YGR026W |
| YDR219C | YIL059C | YNL143C | YER174C | YKL039W |
| YML100W-A | YER156C | YPR092W | YMR068W | YHL046C |
| YMR057C | YER181C | YIL077C | YIL093C | YOR124C |
| YLL012W | YJL028W | YLR059C | YBR191W | YLR123C |
| YGR189C | YIL113W | YCL049C | YGL034C | YPR021C |
| YBR033W | YDL026W | YKL090W | YOL153C | YLR404W |
| YFR012W | YGR230W | YJL100W | YMR144W | YFL034W |
| YGL041C | YHR096C | YMR251W-A | YML109W | YLR173W |
| YOL019W | YNR015W | YAL061W | YCL042W | YPL171C |
| YPL212C | YJL164C | YPL150W | YHR125W | YGR022C |
| YFL044C | YPL201C | YOR243C | YOR178C | YDR445C |
| YLR380W | YKL001C | YER187W | YMR306W | YMR176W |
| YDR491C | YNR039C | YAR020C | YPL203W | YIL173W |
| YBR045C | YHL037C | YHR179W | YGR107W | YDR522C |
| YKL121W | YPR117W | YOR165W | YOL037C | YHR059W |
| YER166W | YDR278C | YER048C | YNR029C | YHL032C |
| YJL059W | YLR311C | YMR202W | YDR426C | YBR245C |
| YDL024C | YBL010C | YDR094W | YIR019C | YLR040C |
| YBR073W | YBR170C | YGR139W | YPL077C | YGR019W |
| YOR091W | YGL117W | YKL149C | YLR328W | YDL093W |
| YAL004W | YIL159W | YBR139W | YIL145C | YMR164C |
| YBL009W | YER075C | YDR344C | YER106W | YLL057C |
| YLR180W | YDL187C | YKR052C | YFL048C | YJL042W |
| YCR107W | YPL196W | YMR320W | YPL254W | YDR474C |
| YGL162W | YFL040W | YMR246W | YOL052C-A | YPL053C |
| YBL048W | YER097W | YER053C | YBR006W | YOR315W |
| YML051W | YOR313C | YBR270C | YDL019C | YNL043C |
| YLR187W | YIL054W | YOR285W | YMR210W | YIL085C |
| YOR344C | YOR381W-A | YLR213C | YHR181W | YBL066C |
| YLR281C | YKR053C | YML050W | YGL131C | YNR002C |
| YDL005C | YPR014C | YAR035W | YER096W | YIL162W |
| YGL082W | YGR294W | YIL029C | YOL007C | YGL035C |
| YAR031W | YNR022C | YGL004C | YPR090W | YLR136C |
| YNL065W | YML020W | YGR233C | YIL105C | YCR100C |
| YNL154C | YJL051W | YBR205W | YOR346W | YPR138C |
| YDL219W | YDR352W | YLR391W | YOL124C | YDR089W |
| YBL106C | YGL166W | YPL048W | YLL054C | YHR073W |
| YDL089W | YER089C | YHR017W | YKR033C | YBR293W |
| YOR050C | YMR012W | YOR190W | YBR178W | YLR349W |
| YAR040C | YMR316C-B | YLR248W | YBR052C | YML054C |
| YPR077C | YFL050C | YGR269W | YMR110C | YDL224C |
| YOR121C | YIL139C | YLR041W | YLR150W | YML074C |

| | | | | |
|---|---|---|---|---|
| YGL164C | YNL175C | YHR132W-A | YLL059C | YJR154W |
| YDR229W | YOR233W | YNL063W | YLL053C | YKL100C |
| YHL016C | YDL188C | YGL215W | YPL108W | YGR087C |
| YMR053C | YFL046W | YHR108W | YLR308W | YDR171W |
| YDR205W | YKL147C | YKL105C | YFR048W | YOR288C |
| YHR039C | YOR300W | YDR098C | YER047C | YBR218C |
| YOR084W | YLR407W | YBR147W | YLR454W | YAL029C |
| YOL016C | YPL246C | YPR071W | YBR008C | YOR238W |
| YER109C | YMR232W | YLR289W | YOR162C | YHR021W-A |
| YBR290W | YOR355W | YOR133W | YDR520C | YBR162W-A |
| YKL033W-A | YOL126C | YMR085W | YAR044W | YLR219W |
| YDR135C | YOR267C | YCR101C | YOR047C | YHL013C |
| YBL065W | YBR116C | YGR070W | YBR201W | YOL099C |
| YMR054W | YNR042W | YKL157W | YOL020W | YOR172W |
| YBR050C | YDR250C | YMR280C | YDR120C | YBL107C |
| YDR451C | YOR314W | YOR345C | YDR381C-A | YDR441C |
| YDR467C | YGR288W | YER051W | YBL036C | YKR097W |
| YGL209W | YGR011W | YKL115C | YKR093W | YDR370C |
| YHL047C | YDR020C | YGL002W | YFL028C | YCL022C |
| YGL033W | YNL027W | YGL017W | YEL048C | YCR102C |
| YGR212W | YLR460C | YAL054C | YDL175C | YOR351C |
| YJL084C | YGR122C-A | YML104C | YCL040W | YKR017C |
| YGR143W | YKL061W | YBL043W | YOL084W | YIR029W |
| YBR069C | YPL032C | YHR029C | YFL047W | YJL058C |
| YBR186W | YML042W | YBR067C | YML004C | YFR030W |
| YDR214W | YKL114C | YIR027C | YKL130C | YKR041W |
| YDR102C | YIL035C | YBL100C | YOR138C | YGR153W |
| YLR044C | YKL117W | YGL197W | YDR133C | YOL073C |
| YPL109C | YLR446W | YLL055W | YNL053W | YDR380W |
| YJL106W | YOL104C | YML053C | YPL226W | YBR066C |
| YFL063W | YMR262W | YCR098C | YOL162W | YKL029C |
| YKR080W | YDL056W | YKL158W | YKL140W | YBR262C |
| YPL004C | YBL070C | YIL100W | YMR001C-A | YMR031C |
| YPR196W | YNL146C-A | YLR408C | YMR107W | YDL124W |
| YLR164W | YKL046C | YFR047C | YHR092C | YKL123W |
| YOL151W | YLR353W | YBR027C | YDR391C | YOL101C |
| YJL105W | YLR236C | YDR287W | YKL215C | YDL214C |
| YER123W | YJL216C | YMR008C | YKR003W | YMR316W |
| YGR035C | YDR161W | YOR273C | YNL204C | YGL250W |
| YGL132W | YPR158W | YJR001W | YGL121C | YMR294W-A |
| YGR126W | YML070W | YPR058W | YJR149W | YJR151C |
| YKR036C | YJL197W | YGR010W | YLR092W | YIL043C |
| YOR088W | YGR018C | YDR502C | YKL174C | YDL189W |
| YIL117C | YLR131C | YDR505C | YOL106W | YDR130C |
| YJR038C | YKL131W | YLR415C | YPL200W | YPL039W |
| YMR178W | YDR387C | YKR106W | YIL123W | YMR010W |

| | | | | |
|---|---|---|---|---|
| YOL053W | YGR254W | YML009C-A | YMR304C-A | YPR083W |
| YOR379C | YDR358W | YLR387C | YDR169C | YOR170W |
| YCR068W | YPL183C | YOL014W | YLR255C | YDR263C |
| YER175W-A | YPL223C | YER121W | YBR296C | YNL135C |
| YIL025C | YAL060W | YGR136W | YCL027W | YOR343C |
| YGL229C | YGR106C | YOR192C | YPR148C | YDR209C |
| YOL136C | YER129W | YBL017C | YHR028C | YGL007W |
| YJR137C | YGR066C | YJL150W | YML118W | YER163C |
| YDR321W | YML021C | YDR419W | YGR194C | YHR109W |
| YNL299W | YGR067C | YMR258C | YKL070W | YML123C |
